# Supplementary material for: Recovering pulsar periodicity from time of arrival data by finding the shortest vector in a lattice
Source: arXiv:2402.07228 source file (2024-11-11)
Supplement: Supplementary file 2 [file second_derivative_tradeoff.tex]

now we understand that the complexity of the algorithm is $\Lambda ^ {a (\sigma)}$ (for a given length $\sigma$), we can predict which high order derivatives are to be included.
For example, with orbital frequency, $C(\text{only orbital frequency, no derivatives}) = (A/dt)^{2a} * N_{\omega}$
\begin{equation}
    \Lambda_1 (\text{first order}) = (A/dt)^{2a} (\Delta_1 \omega / (\delta \omega))^{2a}
\end{equation}
\begin{equation}
    \Lambda_2 (\text{second order}) = (A/dt)^{2a} (\Delta_1 \omega / (\delta \omega))^{2a} (\Delta_2 \omega / (\Delta1\omega))^{4a}
\end{equation}

if $a< 0.5$ you should use at least first order.

if $a<0.25$ you should use at least second order.
